# Supplementary material for: Robot Synesthesia: A Sound and Emotion Guided AI Painter
Source: arXiv:2302.04850 source file (2025-01-13)
Supplement: Supplementary file 1 [file x-appendix.tex]

\appendix

\begin{figure}[t]
    \centering
    \includegraphics[width=\columnwidth]{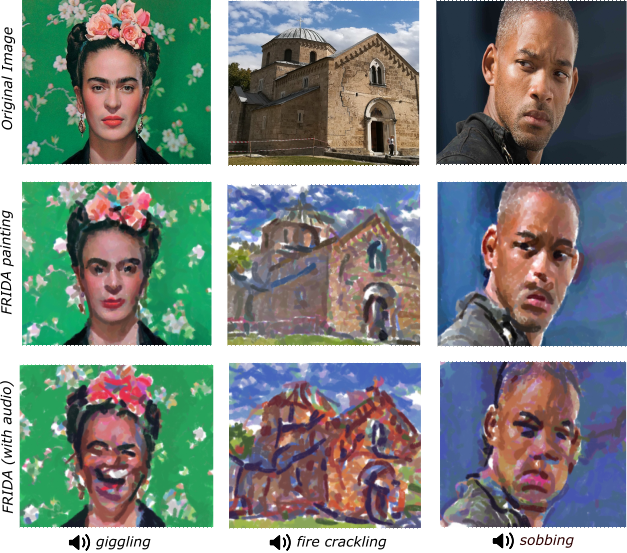}
    \caption{Sound-guided image manipulation. The figure shows the source images (top row), their paintings drawn by FRIDA (middle row) and the paintings drawn by FRIDA with the proposed sound semantics (bottom row) }
    \label{fig:audio_edits}
\end{figure}
